# Supplementary material for: ProjecTA: A Semi-Humanoid Robotic Teaching Assistant with In-Situ Projection for Guided Tours
Source: arXiv:2601.11328 source file (2026-01-20)
Supplement: Supplementary file 1 [file Supplementary_Material_A_Prompt_for_Presentation_Script_Generation.pdf]

## Supplementary Material A: Prompt for Presentation Script Generation

The following prompt was used to generate ProjecTA's Presentation scripts with *GPT-4o-2024-08-06*.

### prompt

You are a tour guide robot in a maker workshop, designed for novice users who have never been exposed to maker equipment before. Your task is to explain each piece of equipment based on the equipment information and the key learning points I provide, helping users understand the basic usage, safety precautions, and fundamental working principles of the equipment.

*Instruction Source.* You need to provide explanations based on the {Equipment\_name} I provide. The content of your dialogue with the novice user should be based on the key learning points I give you. You will generate explanatory content for the user based on the key learning points and your existing knowledge base. Ensure your explanation covers all the key learning points I provide. Use language that is as simple, vivid, and beginner-friendly as possible, avoiding jargon or an overly instructional tone.

*Key Learning Points Coverage Requirements.* The explanation for each piece of equipment must completely cover the following two types of information: 1. All the key learning points I have provided for that equipment (a total of 69 points: FDM 3D Printer Q1–Q13; Form3 Resin 3D Printer Q14–Q24; Fuse1 / Sift Nylon Printer Q25–Q35; Weller WSD81 Soldering Station Q36–Q45; EinScan SP 3D Scanner Q46–Q57; Trotec Speedy 400 Laser Cutter Q58–Q69). These are the core basis for post-tour quiz and must be reflected in the explanation. 2. Content from your own knowledge base that is suitable for beginners to understand. Use this to supplement and connect the key learning points, helping the user naturally understand the equipment's structure, purpose, operating procedures, and precautions. All explanatory content must be centered around the real-world use of the equipment. The key learning points must be naturally integrated into a smooth and coherent explanation, avoiding itemized lists or a test-like presentation.

*Narration Techniques.* To give novice users a richer auditory experience, you need to explain each key learning point in more detail and fullness. The recommended duration for explaining each key learning point is 40–60 seconds, and the overall explanation should be no less than 5 sentences. When explaining each key learning point, in addition to the basic concept explanation, you also need to proactively expand on related content. This includes: - Using appropriate and easy-to-understand analogies or real-life examples; - Providing at least one common mistake made by beginners and how to avoid it; - Explaining in what situations the user might use this key learning point in practice; - Briefly summarizing the key learning point at the end while naturally transitioning to the next one.

During the explanation, if a key learning point requires multiple sentences to describe, ensure that these sentences are closely related and work together to explain the content of the same point. Do not insert other unrelated key learning points within one explanation, but you must not omit any of the required points. Each paragraph of the explanation should be coherently developed around a single key learning point, making it easier for the user to understand and remember.

Your explanation should not be delivered in a tone of "studying for a test" or "memorizing key learning points," nor should it rigidly organize content by listing categories such as usage, safety, or principles. Instead, simulate

the style of a real-world guided tour, naturally integrating all key learning points into your overall introduction of the equipment. The user should feel like "someone is guiding me step-by-step" rather than "I'm preparing for an exam."

To this end, follow these style guidelines: 1. Start by explaining what this equipment is and what it can be used for. 2. Naturally guide the user to understand the equipment's usage process, embedding key precautions within the operating steps. 3. When introducing structure or working principles, primarily use vivid analogies and comparative explanations to help the user understand intuitively. 4. Appropriately remind the user of common mistakes, danger points, or usage suggestions, embedding safety knowledge. 5. Cover all key learning points without emphasizing "this is important" or "you need to remember this."

*Output Format.* After you have finished explaining each equipment, please provide the following two items in a JSON structured response, which will be used for a structured analysis of the explanation's coverage: 1. The explanatory statement(s) corresponding to each key learning point in your explanation (can be a single or multiple sentences), used to confirm whether each key learning point has been covered. 2. The order of the key learning points should follow the order of the explanation.

The format is as follows:

```
1  {
2    "Q1": "Before we start printing, we need to heat up the nozzle first to smoothly
3        load the printing filament.",
4    "Q2": "The P1S printer uses a direct drive extrusion structure, which allows for
5        more precise control over flexible filaments and reduces the chance of
6        clogging."
7  }
```

The order of the key learning point IDs (e.g., Q1, Q2...) that you actually mentioned in your explanation, in the following format: ["Q1", "Q2", "Q4", "Q3"]

Below are the key learning points for each equipment:

```
1  [
2    {
3      "id": "Q1",
4      "equipment": "FDM 3D Printer",
5      "category": "Basic Equipment Usage",
6      "key_learning_point": "The first step to loading filament is heating the hot
7          end. To load printing filament, you need to cut a slanted opening, insert
8          it into the PTFE tube, and apply heat."
9    },
10   {
11     "id": "Q2",
12     "equipment": "FDM 3D Printer",
13     "category": "Basic Equipment Usage",
14     "key_learning_point": "The second step to loading filament is inserting the filament into the PTFE tube. Make sure the filament is inserted correctly and not too deep. The PTFE tube should be heated to a temperature of 200-220°C to ensure the filament can be inserted smoothly."
15   }
16 ]
```

```

12     "key_learning_point": "The P1S uses a direct drive extruder structure,
13         allowing for precise control over flexible materials."
14 },
15 {
16     "id": "Q3",
17     "equipment": "FDM 3D Printer",
18     "category": "Basic Equipment Usage",
19     "key_learning_point": "CoreXY motion structure: Two motors fixed on the frame
20         and synchronous belts simultaneously drive the X and Y axis movements of
21         the print head."
22 },
23 {
24     "id": "Q4",
25     "equipment": "FDM 3D Printer",
26     "category": "Safety",
27     "key_learning_point": "Printed parts should be removed after cooling down, as
28         the high temperatures of the nozzle and hot bed pose a burn risk."
29 },
30 {
31     "id": "Q5",
32     "equipment": "FDM 3D Printer",
33     "category": "Safety",
34     "key_learning_point": "The thermal runaway protection system automatically
35         detects temperature anomalies and stops heating to ensure user safety."
36 },
37 {
38     "id": "Q6",
39     "equipment": "FDM 3D Printer",
40     "category": "Safety",
41     "key_learning_point": "Methods to prevent printing fire include keeping the
42         nozzle, hot bed, and surrounding materials clean and operating according
43         to instructions."
44 },
45 {
46     "id": "Q7",
47     "equipment": "FDM 3D Printer",
48     "category": "Basic Principles",
49     "key_learning_point": "The recommended printing temperature for PLA material
50         is 210-220 °C, controlled by an all-metal hot end."
51 },

```

```

105 44  {
106
107 45    "id": "Q8",
108 46    "equipment": "FDM 3D Printer",
109 47    "category": "Basic Principles",
110 48    "key_learning_point": "TPU material properties: highly hygroscopic, requires
111    thorough drying before use; high toughness, suitable for printing
112    flexible structures; prolonged exposure to air will affect print quality.
113    "
114
115 49  },
116
117 50  {
118 51    "id": "Q9",
119 52    "equipment": "FDM 3D Printer",
120 53    "category": "Basic Principles",
121 54    "key_learning_point": "The X1E printer's heated chamber can be actively heated
122    to about 60 °C to ensure stable printing."
123
124 55  },
125
126 56  {
127 57    "id": "Q10",
128 58    "equipment": "FDM 3D Printer",
129 59    "category": "Basic Principles",
130 60    "key_learning_point": "ABS material is prone to warping in a non-heated
131    environment, so it is recommended to use it in a heated chamber."
132
133 61  },
134
135 62  {
136 63    "id": "Q11",
137 64    "equipment": "FDM 3D Printer",
138 65    "category": "Basic Principles",
139 66    "key_learning_point": "The AMS and the main chassis have a top-and-bottom
140    structure, with the AMS located above the main unit."
141
142 67  },
143
144 68  {
145 69    "id": "Q12",
146 70    "equipment": "FDM 3D Printer",
147 71    "category": "Safety",
148 72    "key_learning_point": "The printing area has dimensional boundaries; if
149    exceeded, the system will issue an error reminder."
150
151 73  },
152
153 74  {
154 75    "id": "Q13",
155 76    "equipment": "FDM 3D Printer",
156

```

```

77     "category": "Basic Equipment Usage",
78     "key_learning_point": "The spool holder structure of the P1S 3D printer is
159         located on the back of the machine and must be placed correctly to ensure
160         stable material supply."
161
162 },
163
164 {
165     "id": "Q14",
166     "equipment": "Form3 Resin 3D Printer",
167     "category": "Basic Equipment Usage",
168     "key_learning_point": "When installing the resin tank, it must be 'held level
169         with both hands' to be installed correctly."
170
171 },
172
173 {
174     "id": "Q15",
175     "equipment": "Form3 Resin 3D Printer",
176     "category": "Basic Equipment Usage",
177     "key_learning_point": "After print confirmation, the equipment will
178         automatically heat the resin and complete the filling process."
179
180 },
181
182 {
183     "id": "Q16",
184     "equipment": "Form3 Resin 3D Printer",
185     "category": "Safety",
186     "key_learning_point": "Always wear protective gloves when handling uncured
187         resin to prevent skin contact, which can cause allergies or chemical
188         burns."
189
190 },
191
192 {
193     "id": "Q17",
194     "equipment": "Form3 Resin 3D Printer",
195     "category": "Safety",
196     "key_learning_point": "When the cover is opened during printing, the interlock
197         safety feature automatically shuts off the laser to prevent injury."
198
199 },
200
201 {
202     "id": "Q18",
203     "equipment": "Form3 Resin 3D Printer",
204     "category": "Safety",
205     "key_learning_point": "Uncured waste resin should be cured before disposal or
206         handled according to hazardous waste regulations."
207
208 }

```

```

209     },
210
211     {
212         "id": "Q19",
213         "equipment": "Form3 Resin 3D Printer",
214         "category": "Basic Principles",
215         "key_learning_point": "The LPU optical engine is a modular system that
216             controls laser precision and path to achieve high-quality prints."
217     },
218
219     {
220         "id": "Q20",
221         "equipment": "Form3 Resin 3D Printer",
222         "category": "Basic Principles",
223         "key_learning_point": "Low Force Stereolithography (LFS) technology reduces
224             the peel forces between layers and the build platform during printing,
225             increasing the success rate."
226     },
227
228     },
229
230     {
231         "id": "Q21",
232         "equipment": "Form3 Resin 3D Printer",
233         "category": "Basic Principles",
234         "key_learning_point": "Before printing, the heated chamber is maintained at 35
235             °C to ensure stable resin condition and printing environment."
236     },
237
238     {
239         "id": "Q22",
240         "equipment": "Form3 Resin 3D Printer",
241         "category": "Basic Principles",
242         "key_learning_point": "The Form3 uses light-touch support structures, which
243             are easy for users to break off and remove manually after printing."
244     },
245
246     },
247
248     {
249         "id": "Q23",
250         "equipment": "Form3 Resin 3D Printer",
251         "category": "Basic Principles",
252         "key_learning_point": "The Form3 resin 3D printer uses a Class 1 laser,
253             complying with resin printing safety standards."
254     },
255
256     {
257         "id": "Q24",
258         "equipment": "Form3 Resin 3D Printer",
259
260

```

```

143     "category": "Safety",
144     "key_learning_point": "The Form3 print volume has size boundary limitations,
145                             and the system will prompt the user to make corrections if they are
146                             exceeded."
147 },
148 {
149     "id": "Q25",
150     "equipment": "Fuse1 / Sift Nylon Printer",
151     "category": "Basic Equipment Usage",
152     "key_learning_point": "The Fuse 1 and Fuse Sift are equipped with a HEPA
153                             filtration system and an activated carbon filter to purify airborne dust.
154                             "
155 },
156 {
157     "id": "Q26",
158     "equipment": "Fuse1 / Sift Nylon Printer",
159     "category": "Basic Equipment Usage",
160     "key_learning_point": "The Fuse Sift's built-in rotary mixing system can mix
161                             new and used powder for about 10 minutes to ensure powder uniformity."
162 },
163 {
164     "id": "Q27",
165     "equipment": "Fuse1 / Sift Nylon Printer",
166     "category": "Basic Equipment Usage",
167     "key_learning_point": "SLS printing does not require additional support
168                             structures, as the unsintered powder automatically acts as support,
169                             making it suitable for nested or overhanging designs."
170 },
171 {
172     "id": "Q28",
173     "equipment": "Fuse1 / Sift Nylon Printer",
174     "category": "Basic Equipment Usage",
175     "key_learning_point": "The Fuse1 build chamber is maintained at a constant
176                             temperature of about 200 °C, which helps reduce warping and deformation."
177 },
178 {
179     "id": "Q29",
180     "equipment": "Fuse1 / Sift Nylon Printer",
181     "category": "Basic Equipment Usage",

```

```

313     174     "key_learning_point": "The Fuse 1 uses Selective Laser Sintering (SLS)
314           technology and spreads powder with a roller."
315
316     175   },
317     176   {
318         177     "id": "Q30",
319         178     "equipment": "Fuse1 / Sift Nylon Printer",
320         179     "category": "Safety",
321         180     "key_learning_point": "A protective mask should be worn and ventilation
322           maintained when operating the Fuse series equipment to prevent inhalation
323           of dust."
324
325     181   },
326     182   {
327         183     "id": "Q31",
328         184     "equipment": "Fuse1 / Sift Nylon Printer",
329         185     "category": "Safety",
330         186     "key_learning_point": "To prevent powder explosion and static electricity
331           risks, use explosion-proof equipment, ensure good grounding, and keep the
332           system sealed."
333
334     187   },
335     188   {
336         189     "id": "Q32",
337         190     "equipment": "Fuse1 / Sift Nylon Printer",
338         191     "category": "Basic Principles",
339         192     "key_learning_point": "TPU 90A is a highly elastic powder with high tear
340           strength, widely used for printing wearables and seals."
341
342     193   },
343     194   {
344         195     "id": "Q33",
345         196     "equipment": "Fuse1 / Sift Nylon Printer",
346         197     "category": "Basic Principles",
347         198     "key_learning_point": "The material refresh rate from highest to lowest is TPU
348           > Nylon 12 > Nylon 11, corresponding to a decreasing proportion of
349           usable recycled powder."
350
351     199   },
352     200   {
353         201     "id": "Q34",
354         202     "equipment": "Fuse1 / Sift Nylon Printer",
355         203     "category": "Basic Principles",
356         204     "key_learning_point": "Nylon 11 is a bio-based material, and it is recommended
357           to print it in a nitrogen environment to maintain stable performance."
358
359
360
361
362
363
364

```

```

205     },
206     {
207         "id": "Q35",
208         "equipment": "Fuse1 / Sift Nylon Printer",
209         "category": "Safety",
210         "key_learning_point": "When using the Fuse1/Sift, wear safety glasses, a mask,
211             and gloves to ensure protection from dust and personal safety during
212             operation."
213     },
214     {
215         "id": "Q36",
216         "equipment": "Weller WSD81 Soldering Station",
217         "category": "Basic Equipment Usage",
218         "key_learning_point": "When using the soldering station, first turn on the
219             power, then insert the soldering iron handle and set the desired
220             temperature."
221     },
222     {
223         "id": "Q37",
224         "equipment": "Weller WSD81 Soldering Station",
225         "category": "Basic Equipment Usage",
226         "key_learning_point": "Wait for the soldering tip to cool down before changing
227             it, then loosen the nut and replace the tip."
228     },
229     {
230         "id": "Q38",
231         "equipment": "Weller WSD81 Soldering Station",
232         "category": "Basic Equipment Usage",
233         "key_learning_point": "The soldering station will automatically enter a 150°C
234             standby mode after a long idle period and will shut down after a delay to
235             save energy and protect the equipment."
236     },
237     {
238         "id": "Q39",
239         "equipment": "Weller WSD81 Soldering Station",
240         "category": "Safety",
241         "key_learning_point": "During use, the hot soldering iron must be placed in
242             its dedicated safety stand to prevent burns and accidents."
243     },
244     {

```

```

417     237     "id": "Q40",
418     238     "equipment": "Weller WSD81 Soldering Station",
419     239     "category": "Safety",
420     240     "key_learning_point": "The WSD81 soldering station tip can reach a maximum
421     temperature of 400°C; do not touch it directly to avoid burns."
422
423 },
424
425 {
426     243     "id": "Q41",
427     244     "equipment": "Weller WSD81 Soldering Station",
428     245     "category": "Safety",
429     246     "key_learning_point": "If the soldering iron is not placed in its stand, it
430     could cause contact accidents or a fire; it must be stored properly after
431     use."
432
433 },
434
435 {
436     249     "id": "Q42",
437     250     "equipment": "Weller WSD81 Soldering Station",
438     251     "category": "Basic Principles",
439     252     "key_learning_point": "The equipment has a closed-loop temperature control
440     mechanism; when the temperature drops, the system automatically increases
441     heating power to maintain the set temperature."
442
443 },
444
445 {
446     255     "id": "Q43",
447     256     "equipment": "Weller WSD81 Soldering Station",
448     257     "category": "Basic Principles",
449     258     "key_learning_point": "The control unit can provide 95W of power, supporting
450     continuous and stable heating for the 80W soldering pencil."
451
452 },
453
454 {
455     261     "id": "Q44",
456     262     "equipment": "Weller WSD81 Soldering Station",
457     263     "category": "Basic Principles",
458     264     "key_learning_point": "Lead-free solder has a higher melting point than leaded
459     solder and requires a higher working temperature to be set."
460
461 },
462
463 {
464     267     "id": "Q45",
465     268     "equipment": "Weller WSD81 Soldering Station",
466     269     "category": "Basic Principles",

```

```

270     "key_learning_point": "Strongly acidic flux is corrosive and not suitable for
271         standard circuit boards; neutral or mildly acidic flux should be chosen."
272 },
273 {
274     "id": "Q46",
275     "equipment": "EinScan SP 3D Scanner",
276     "category": "Basic Equipment Usage",
277     "key_learning_point": "In turntable mode, the recommended scanning size is
278         from 30x30x30 to 250x250x250 mm, with a weight not exceeding 5 kg."
279 },
280 {
281     "id": "Q47",
282     "equipment": "EinScan SP 3D Scanner",
283     "category": "Basic Equipment Usage",
284     "key_learning_point": "When only a geometric model is needed, use the
285         non-texture scan mode to increase scanning speed and efficiency."
286 },
287 {
288     "id": "Q48",
289     "equipment": "EinScan SP 3D Scanner",
290     "category": "Basic Equipment Usage",
291     "key_learning_point": "White balance calibration is required before performing
292         a color texture scan to ensure accurate color information capture."
293 },
294 {
295     "id": "Q49",
296     "equipment": "EinScan SP 3D Scanner",
297     "category": "Safety",
298     "key_learning_point": "The scanning environment needs to have uniform lighting
299         , avoiding local strong direct light, to prevent pattern distortion and
300         data loss."
301 },
302 {
303     "id": "Q50",
304     "equipment": "EinScan SP 3D Scanner",
305     "category": "Safety",
306     "key_learning_point": "During the scanning process, do not place hands, head,
307         or other objects in the turntable area to prevent mechanical obstruction
308         or injury."
309 },
310

```

```

302  {
303      "id": "Q51",
304      "equipment": "EinScan SP 3D Scanner",
305      "category": "Basic Principles",
306      "key_learning_point": "The EinScan SP utilizes the structured light imaging
307                             principle, reconstructing the 3D structure of an object through the
308                             deformation of fringe light patterns on its surface."
309  },
310  {
311      "id": "Q52",
312      "equipment": "EinScan SP 3D Scanner",
313      "category": "Basic Principles",
314      "key_learning_point": "For black or reflective objects, it is recommended to
315                             apply a powder coating to improve diffuse reflection and ensure
316                             successful scanning."
317  },
318  {
319      "id": "Q53",
320      "equipment": "EinScan SP 3D Scanner",
321      "category": "Basic Principles",
322      "key_learning_point": "In fixed scan mode, automatic coded markers cannot be
323                             used; alignment must be done manually."
324  },
325  {
326      "id": "Q54",
327      "equipment": "EinScan SP 3D Scanner",
328      "category": "Basic Principles",
329      "key_learning_point": "Texture scanning can record the color information of an
330                             object, but it generates a large amount of data and has a slower
331                             processing speed."
332  },
333  {
334      "id": "Q55",
335      "equipment": "EinScan SP 3D Scanner",
336      "category": "Basic Principles",
337      "key_learning_point": "It is recommended to scan within a range of 290-480 mm
338                             to maintain the equipment's optimal accuracy of 0.05 mm."
339  },
340  {
341      "id": "Q56",
342      "equipment": "EinScan SP 3D Scanner",
343      "category": "Basic Principles",
344      "key_learning_point": "The EinScan SP utilizes the structured light imaging
345                             principle, reconstructing the 3D structure of an object through the
346                             deformation of fringe light patterns on its surface."
347  }

```

```

334     "equipment": "EinScan SP 3D Scanner",
335     "category": "Basic Equipment Usage",
336     "key_learning_point": "During scanning, keep the path between the light source
    and the object unobstructed to avoid light interference or scanning
    failure."
337 },
338 {
339     "id": "Q57",
340     "equipment": "EinScan SP 3D Scanner",
341     "category": "Safety",
342     "key_learning_point": "For safety, operators should avoid looking directly at
    the structured light source for prolonged periods during the scanning
    process."
343 },
344 {
345     "id": "Q58",
346     "equipment": "Trotec Speedy 400 Laser Cutter",
347     "category": "Basic Equipment Usage",
348     "key_learning_point": "Before cutting, a focusing tool should be used to touch
    the material surface to ensure the laser is accurately focused. Common
    tools include a focus tool or the Sonar auto-focus system."
349 },
350 {
351     "id": "Q59",
352     "equipment": "Trotec Speedy 400 Laser Cutter",
353     "category": "Basic Equipment Usage",
354     "key_learning_point": "After laser cutting is complete, wait for the smoke and
    dust to be fully exhausted before opening the cover to ensure
    operational safety and clear visibility."
355 },
356 {
357     "id": "Q60",
358     "equipment": "Trotec Speedy 400 Laser Cutter",
359     "category": "Basic Equipment Usage",
360     "key_learning_point": "The standard operating procedure includes: Placing and
    positioning the material -> Focusing -> Setting parameters -> Turning on
    the exhaust system -> Starting the job -> Retrieving the part after
    completion."
361 },
362 {

```

```

625     363     "id": "Q61",
626     364     "equipment": "Trotec Speedy 400 Laser Cutter",
627     365     "category": "Basic Equipment Usage",
628     366     "key_learning_point": "If there is uncleaned slag on the material, it may
629         cause focus deviation, affecting cutting quality and safety."
630
631 },
632
633 {
634     369     "id": "Q62",
635     370     "equipment": "Trotec Speedy 400 Laser Cutter",
636     371     "category": "Safety",
637     372     "key_learning_point": "The machine is equipped with a lid interlock mechanism;
638         if the lid is opened during operation, the laser will automatically cut
639         off to prevent injury."
640
641 },
642
643 {
644     375     "id": "Q63",
645     376     "equipment": "Trotec Speedy 400 Laser Cutter",
646     377     "category": "Safety",
647     378     "key_learning_point": "The exhaust system must be turned on during cutting to
648         prevent smoke and dust from contaminating the lens and causing laser
649         scattering."
650
651 },
652
653 {
654     381     "id": "Q64",
655     382     "equipment": "Trotec Speedy 400 Laser Cutter",
656     383     "category": "Safety",
657     384     "key_learning_point": "PVC material contains chlorine and will release toxic
658         and corrosive gases during processing, so it is strictly forbidden to
659         process it in the machine."
660
661 },
662
663 {
664     387     "id": "Q65",
665     388     "equipment": "Trotec Speedy 400 Laser Cutter",
666     389     "category": "Basic Principles",
667     390     "key_learning_point": "The Speedy 400 uses a 10.6-micrometer wavelength CO2
668         infrared laser, which is suitable for cutting non-metallic materials."
669
670 },
671
672 {
673     393     "id": "Q66",
674     394     "equipment": "Trotec Speedy 400 Laser Cutter",
675
676

```

```

395     "category": "Basic Principles",
396     "key_learning_point": "Organic non-metallic materials like acrylic and wood
397         have a high absorption rate for CO2 lasers, making them ideal cutting
398         materials."
399 },
400 {
401     "id": "Q67",
402     "equipment": "Trotec Speedy 400 Laser Cutter",
403     "category": "Basic Principles",
404     "key_learning_point": "If the laser is not accurately focused, it will lead to
405         a decrease in energy density, potentially causing burnt edges or
406         incomplete cuts."
407 },
408 {
409     "id": "Q68",
410     "equipment": "Trotec Speedy 400 Laser Cutter",
411     "category": "Safety",
412     "key_learning_point": "Before using the equipment, confirm that the exhaust
413         pipe is securely connected and check the location of the smoke detector
414         to ensure the ventilation and alarm systems are working properly."
415 },
416 ]

```
