# Supplementary material for: ProjecTA: A Semi-Humanoid Robotic Teaching Assistant with In-Situ Projection for Guided Tours
Source: arXiv:2601.11328 source file (2026-01-20)
Supplement: Supplementary file 2 [file Supplementary_Material_B_Visual_Assets_Orchestration.pdf]

## Supplementary Material B: Prompt for Visual Assets Orchestration

### prompt

You are the “Projection Matching Agent,” responsible for projecting corresponding line drawings or GIF Stickers in real time according to the teaching content.

*Input Variables.* {teaching\_content}: The complete instructional text, with each key learning point marked at the end of the sentence using (QX). {knowledge\_sequence}: A list of key learning point identifiers arranged in the order of instruction, e.g., [“Q1”, “Q2”, ...]. assets: A list of available image/GIF resources in JSON array format, where each entry includes filename, location, description, and linked learning point.

*Working Process.* The Projection Matching Agent follows these steps:

**Step 1: Locate Key Learning Points.** Scan {teaching\_content} and locate each sentence containing “(QX),” recording the corresponding key learning point QX for that sentence.

**Step 2: Determine Projection Position.** For each sentence with (QX), retrieve the value of the location field in assets to determine the projection position of the visual asset corresponding to QX.

**Step 3: Projection Display Rules.** Execute the projection display according to the following priority:

(a) *Special GIFs (highest priority).* When the following conditions are detected, the Projection Matching Agent outputs GIF (Rn) in order of priority, and after playback (if a corresponding key learning point QX exists), switches to the visual asset of that key learning point. Otherwise, it retains the current GIF (Rn). The projection location of GIF (Rn) is likewise determined by retrieving the location field associated with RX in assets.

**Prohibitive meaning:** If the sentence contains prohibitive keywords such as “prohibited,” “dangerous,” or “must not,” display R1.gif, which represents the prohibition of dangerous operations and behaviors. After 2 seconds of playback, if the sentence involves a key learning point QX, switch to the corresponding QX visual asset; otherwise, retain R1.

**Cautionary meaning:** If the sentence contains cautionary keywords such as “pay attention,” “be aware,” or “ensure,” display R2.gif, which represents the importance of paying attention. After 2 seconds of playback, if the sentence involves a key learning point QX, switch to the corresponding QX visual asset; otherwise, retain R2.

**At the start of equipment explanation:** (i) FDM 3D Printer, Form3, and EinScan SP: display R5.gif (arrow pointing downward). (ii) Trotec Speedy 400: display R6.gif (arrow pointing rightward). (iii) Fuse1/Sift and Weller WSD81: project either R3.gif or R4.gif (a glowing orb or halo indicating emphasis on a specific object).

**After all key learning points QX have been explained:** Display R7.gif (arrow moving leftward).

(b) *Regular Key Learning Point Visual Asset Display.* If no special GIF is triggered, and QX is included in {knowledge\_sequence}, locate the asset in which the fourth field linked\_learning\_point == QX. Verify whether the key learning point corresponds with the description field of the image. If consistent, output and display it. For example, if Q1 is detected in {knowledge\_sequence}, locate the corresponding visual asset Q1 . jpg and, according to the description field, display: “The first step of loading printing material is heating the hot end.”

(c) *Multiple Visual Asset Display.* If multiple assets correspond to the same key learning point QX, output them sequentially.

*Projection and Speech Duration Estimation.* A large language model is employed to estimate the duration (in seconds) of each text segment when produced as TTS output. The result is recorded as QX(seconds) and stored in a JSON sequence assigned to the variable {knowledgeaudio\_time\_sequence}.

**GIF Duration Rules.** GIFs are detected and triggered in instructional order: R1 (2s), R2 (2s), R5, R6, R3 or R4, and R7. The duration of each Rn is estimated (R1 and R2 are fixed at 2s; others are rounded down to the nearest integer) and recorded as Rn(seconds).

**Combination Rules.** If Rn and QX are triggered simultaneously at the same position, they are combined into Rn(seconds)QX(seconds); otherwise, they are output separately as either Rn(seconds) or QX(seconds).

**Final Output Format.** The final output is a JSON list {projectionaudio\_time\_sequence}, exemplified as:

```
1 [ "R5(15s)", "Q1(23s)", "R1(2s)Q2(30s)", "Q3(18s)", ... ]
```

The following is the JSON description of image and GIF assets:

```
1 [
2   {
3     "filename": "Q1.jpg",
4     "location": "Nearby surfaces of FDM 3D Printer",
5     "description": "The first step to loading filament is heating the hot end (cut
6       a slant, insert into PTFE tube, and heat)",
7     "linked_learning_point": "Q1"
8   },
9   {
10    "filename": "Q2.jpg",
11    "location": "Nearby surfaces of FDM 3D Printer",
12    "description": "Direct drive extrusion for precise control of flexible
13      materials",
14    "linked_learning_point": "Q2"
15  },
16  {
17    "filename": "Q3.jpg",
18    "location": "Nearby surfaces of FDM 3D Printer",
19    "description": "CoreXY motion structure high-speed printing principle",
20    "linked_learning_point": "Q3"
21  },
22  {
23    "filename": "Q4.jpg",
24    "location": "Nearby surfaces of FDM 3D Printer",
25    "description": "Nozzle and hot bed temperatures are high, must cool down
26      before removing the print",
27    "linked_learning_point": "Q4"
28  },
29  ],
```

```

26  {
27      "filename": "Q5.jpg",
28      "location": "Nearby surfaces of FDM 3D Printer",
29      "description": "Thermal runaway protection function Automatic detection, stop
30      heating",
31      "linked_learning_point": "Q5"
32  },
33  {
34      "filename": "Q6.jpg",
35      "location": "Nearby surfaces of FDM 3D Printer",
36      "description": "Moving parts safety + High-temperature protection + Following
37      instructions can prevent fire",
38      "linked_learning_point": "Q6"
39  },
40  {
41      "filename": "Q7.jpg",
42      "location": "Nearby surfaces of FDM 3D Printer",
43      "description": "Different materials require different temperature settings (
44      PLA 210-220 C)",
45      "linked_learning_point": "Q7"
46  },
47  {
48      "filename": "Q8.jpg",
49      "location": "Nearby surfaces of FDM 3D Printer",
50      "description": "TPU material needs to be dried, direct drive extrusion system
51      provides precise control over flexible filament",
52      "linked_learning_point": "Q8"
53  },
54  {
55      "filename": "Q9.jpg",
56      "location": "Nearby surfaces of FDM 3D Printer",
57      "description": "Heated chamber can reach a maximum temperature of about 60 C",
58      "linked_learning_point": "Q9"
59  },
60  {
61      "filename": "Q10.jpg",
62      "location": "Nearby surfaces of FDM 3D Printer",
63      "description": "ABS not recommended for non-heated chambers, ABS warps easily,
64      requires heated environment to prevent deformation",
65      "linked_learning_point": "Q10"

```

```

105     },
106
107     {
108         "filename": "Q11.jpg",
109         "location": "Nearby surfaces of FDM 3D Printer",
110         "description": "Automatic Material System (AMS) structure and relative
111             position to the main unit",
112         "linked_learning_point": "Q11"
113     },
114
115     {
116         "filename": "Q12.jpg",
117         "location": "Nearby surfaces of FDM 3D Printer",
118         "description": "Printable size range is limited, be careful not to exceed the
119             printable dimensions",
120         "linked_learning_point": "Q12"
121     },
122
123     {
124         "filename": "Q13.jpg",
125         "location": "Nearby surfaces of FDM 3D Printer",
126         "description": "Position and structure of the spool holder on the back of the
127             FDM 3D printer",
128         "linked_learning_point": "Q13"
129     },
130
131     {
132         "filename": "Q14.jpg",
133         "location": "Nearby surfaces of Form3 Resin 3D Printer ",
134         "description": "Installing the resin tank requires holding it level with both
135             hands to ensure proper installation",
136         "linked_learning_point": "Q14"
137     },
138
139     {
140         "filename": "Q15.jpg",
141         "location": "Nearby surfaces of Form3 Resin 3D Printer ",
142         "description": "Automatic resin heating and filling function before printing",
143         "linked_learning_point": "Q15"
144     },
145
146     {
147         "filename": "Q16.jpg",
148         "location": "Nearby surfaces of Form3 Resin 3D Printer ",
149         "description": "Always wear protective gloves when handling uncured resin",
150         "linked_learning_point": "Q16"
151     }
152
153
154
155
156

```

```

97     },
98     {
99         "filename": "Q17.jpg",
100         "location": "Nearby surfaces of Form3 Resin 3D Printer ",
101         "description": "Laser automatically turns off if the cover is opened during
102             printing, the printer cover has an interlock safety device",
103         "linked_learning_point": "Q17"
104     },
105     {
106         "filename": "Q18.jpg",
107         "location": "Nearby surfaces of Form3 Resin 3D Printer ",
108         "description": "Waste resin disposal method uncured waste resin should be
109             cured before disposal or treated as hazardous waste",
110         "linked_learning_point": "Q18"
111     },
112     {
113         "filename": "Q19.jpg",
114         "location": "Nearby surfaces of Form3 Resin 3D Printer ",
115         "description": "Light Processing Unit (LPU) function Controls laser precision
116             and path",
117         "linked_learning_point": "Q19"
118     },
119     {
120         "filename": "Q20.jpg",
121         "location": "Nearby surfaces of Form3 Resin 3D Printer ",
122         "description": "Main advantage of Low Force Stereolithography (LFS) technology
123             Increases print success rate",
124         "linked_learning_point": "Q20"
125     },
126     {
127         "filename": "Q21.jpg",
128         "location": "Nearby surfaces of Form3 Resin 3D Printer ",
129         "description": "Heated chamber maintains 35 C before printing",
130         "linked_learning_point": "Q21"
131     },
132     {
133         "filename": "Q22.jpg",
134         "location": "Nearby surfaces of Form3 Resin 3D Printer ",
135         "description": "Support structure generation light-touch supports, easy to
136             remove manually",

```

```

209     "linked_learning_point": "Q22"
210 },
211 {
212     "filename": "Q23.jpg",
213     "location": "Nearby surfaces of Form3 Resin 3D Printer ",
214     "description": "Form3 resin 3D printer laser safety class is Class 1",
215     "linked_learning_point": "Q23"
216 },
217 {
218     "filename": "Q24.jpg",
219     "location": "Nearby surfaces of Form3 Resin 3D Printer ",
220     "description": "Overall device dimensions are approx 40x38x55 cm, max
221     printable size is 14.5x14.5x18.5 cm",
222     "linked_learning_point": "Q24"
223 },
224 {
225     "filename": "Q25.jpg",
226     "location": "Nearby surfaces of Fuse1 / Sift Nylon Printer ",
227     "description": "Fuse 1 and Fuse Sift are equipped with HEPA air filtration
228     system and activated carbon filter",
229     "linked_learning_point": "Q25"
230 },
231 {
232     "filename": "Q26.jpg",
233     "location": "Nearby surfaces of Fuse1 / Sift Nylon Printer ",
234     "description": "Fuse Sift has a built-in rotary mixing system that can mix new
235     and used powder for about 10 minutes",
236     "linked_learning_point": "Q26"
237 },
238 {
239     "filename": "Q27.jpg",
240     "location": "Nearby surfaces of Fuse1 / Sift Nylon Printer ",
241     "description": "Selective Laser Sintering (SLS) does not require support
242     structures, unsintered powder acts as support, allowing direct printing
243     of nested or overhanging structures",
244     "linked_learning_point": "Q27"
245 },
246 {
247     "filename": "Q28.jpg",
248     "location": "Nearby surfaces of Fuse1 / Sift Nylon Printer ",
249     "description": "Selective Laser Sintering (SLS) does not require support
250     structures, unsintered powder acts as support, allowing direct printing
251     of nested or overhanging structures",
252     "linked_learning_point": "Q27"
253 },
254 {
255     "filename": "Q28.jpg",
256     "location": "Nearby surfaces of Fuse1 / Sift Nylon Printer ",
257     "description": "Selective Laser Sintering (SLS) does not require support
258     structures, unsintered powder acts as support, allowing direct printing
259     of nested or overhanging structures",
260     "linked_learning_point": "Q27"

```

```

167     "description": "Build chamber maintains constant temperature of about 200 C
168         for sintering printing at near-melting temperatures reduces warping",
169     "linked_learning_point": "Q28"
170 },
171 {
172     "filename": "Q29.jpg",
173     "location": "Nearby surfaces of Fuse1 / Sift Nylon Printer ",
174     "description": "Fuse 1 uses Selective Laser Sintering (SLS) principle and a
175         roller powder spreading mechanism",
176     "linked_learning_point": "Q29"
177 },
178 {
179     "filename": "Q30.jpg",
180     "location": "Nearby surfaces of Fuse1 / Sift Nylon Printer ",
181     "description": "Dust protection wear a mask when handling powder, maintain
182         ventilation to prevent inhalation",
183     "linked_learning_point": "Q30"
184 },
185 {
186     "filename": "Q31.jpg",
187     "location": "Nearby surfaces of Fuse1 / Sift Nylon Printer ",
188     "description": "Preventing static and dust explosions please use special
189         gloves and a sealed equipment cleaning system",
190     "linked_learning_point": "Q31"
191 },
192 {
193     "filename": "Q32.jpg",
194     "location": "Nearby surfaces of Fuse1 / Sift Nylon Printer ",
195     "description": "TPU 90A elastomeric powder with high elasticity and high tear
196         strength, suitable for wearables, seals, etc.",
197     "linked_learning_point": "Q32"
198 },
199 {
200     "filename": "Q33.jpg",
201     "location": "Nearby surfaces of Fuse1 / Sift Nylon Printer ",
202     "description": "Material refresh rate TPU<Nylon 12<Nylon 11 (usable recycled
203         powder ratio decreases accordingly)",
204     "linked_learning_point": "Q33"
205 },
206 {

```

```

313 201     "filename": "Q34.jpg",
314 202     "location": "Nearby surfaces of Fuse1 / Sift Nylon Printer ",
315 203     "description": "Nylon 11 is recommended to be printed in a nitrogen
316 204         environment to maintain performance stability",
317 205     "linked_learning_point": "Q34"
318 206 },
319 207 {
320 208     "filename": "Q35.jpg",
321 209     "location": "Nearby surfaces of Fuse1 / Sift Nylon Printer ",
322 210     "description": "Safety regulations wear safety glasses, mask, and gloves
323 211         during operation",
324 212     "linked_learning_point": "Q35"
325 213 },
326 214 {
327 215     "filename": "Q36.jpg",
328 216     "location": "Nearby surfaces of Weller WSD81 Soldering Station ",
329 217     "description": "Power-on and temperature setting turn on power, then insert
330 218         soldering iron handle and adjust temperature",
331 219     "linked_learning_point": "Q36"
332 220 },
333 221 {
334 222     "filename": "Q37.jpg",
335 223     "location": "Nearby surfaces of Weller WSD81 Soldering Station ",
336 224     "description": "Soldering tip installation and removal cool down, then loosen
337 225         the nut and replace the tip",
338 226     "linked_learning_point": "Q37"
339 227 },
340 228 {
341 229     "filename": "Q38.jpg",
342 230     "location": "Nearby surfaces of Weller WSD81 Soldering Station ",
343 231     "description": "Soldering iron enters 150 C standby after long idle period",
344 232     "linked_learning_point": "Q38"
345 233 },
346 234 {
347 235     "filename": "Q39.jpg",
348 236     "location": "Nearby surfaces of Weller WSD81 Soldering Station ",
349 237     "description": "Burn prevention soldering iron must be placed in safety stand
350 238         during operation",
351 239     "linked_learning_point": "Q39"
352 240 },
353 241 },
354 242 {
355 243     "filename": "Q39.jpg",
356 244     "location": "Nearby surfaces of Weller WSD81 Soldering Station ",
357 245     "description": "Burn prevention soldering iron must be placed in safety stand
358 246         during operation",
359 247     "linked_learning_point": "Q39"
360 248 },
361 249 },
362 250 },
363 251 },
364 252 }

```

```

236 {
237     "filename": "Q40.jpg",
238     "location": "Nearby surfaces of Weller WSD81 Soldering Station ",
239     "description": "Maximum tip temperature is 400 C, do not touch the hot tip",
240     "linked_learning_point": "Q40"
241 },
242 {
243     "filename": "Q41.jpg",
244     "location": "Nearby surfaces of Weller WSD81 Soldering Station ",
245     "description": "Not placing the iron in its stand could cause a fire",
246     "linked_learning_point": "Q41"
247 },
248 {
249     "filename": "Q42.jpg",
250     "location": "Nearby surfaces of Weller WSD81 Soldering Station ",
251     "description": "Closed-loop temperature control, real-time monitoring and
252         dynamic adjustment of heating power, power automatically increases when
253         temperature drops",
254     "linked_learning_point": "Q42"
255 },
256 {
257     "filename": "Q43.jpg",
258     "location": "Nearby surfaces of Weller WSD81 Soldering Station ",
259     "description": "Control unit provides 95W of power, supplying ample energy for
260         the 80W soldering pencil",
261     "linked_learning_point": "Q43"
262 },
263 {
264     "filename": "Q44.jpg",
265     "location": "Nearby surfaces of Weller WSD81 Soldering Station ",
266     "description": "Lead-free solder has a higher melting point than leaded solder
267         ",
268     "linked_learning_point": "Q44"
269 },
270 {
271     "filename": "Q45.jpg",
272     "location": "Nearby surfaces of Weller WSD81 Soldering Station ",
273     "description": "Strongly acidic flux is corrosive and not suitable for
274         standard circuit boards",
275     "linked_learning_point": "Q45"
276 }

```

```

417     },
418
419     {
420         "filename": "Q46.jpg",
421         "location": "Nearby surfaces of EinScan SP 3D Scanner ",
422         "description": "Recommended scanning size range (turntable mode) automatic
423             scanning range up to approx 200x200x200 mm, weight <= 5 kg",
424         "linked_learning_point": "Q46"
425     },
426
427     {
428         "filename": "Q47.jpg",
429         "location": "Nearby surfaces of EinScan SP 3D Scanner ",
430         "description": "Use non-texture scan mode when only a geometric model is
431             needed",
432         "linked_learning_point": "Q47"
433     },
434
435     {
436         "filename": "Q48.jpg",
437         "location": "Nearby surfaces of EinScan SP 3D Scanner ",
438         "description": "White balance calibration is required before texture scanning
439             mode to ensure accurate color capture",
440         "linked_learning_point": "Q48"
441     },
442
443     {
444         "filename": "Q49.jpg",
445         "location": "Nearby surfaces of EinScan SP 3D Scanner ",
446         "description": "Maintain uniform lighting to avoid local bright spots",
447         "linked_learning_point": "Q49"
448     },
449
450     {
451         "filename": "Q50.jpg",
452         "location": "Nearby surfaces of EinScan SP 3D Scanner ",
453         "description": "Do not place hands, head, or objects in the scanning area to
454             prevent turntable obstruction or entanglement",
455         "linked_learning_point": "Q50"
456     },
457
458     {
459         "filename": "Q51.jpg",
460         "location": "Nearby surfaces of EinScan SP 3D Scanner ",
461         "description": "Structured light principle is fringe light projection,
462             reconstructing 3D shape through fringe deformation",
463     }
464
465
466
467
468

```

```

306     "linked_learning_point": "Q51"
307 },
308 {
309     "filename": "Q52.jpg",
310     "location": "Nearby surfaces of EinScan SP 3D Scanner ",
311     "description": "Reflective objects have poor reflectivity, require powder
312                   coating to improve diffuse reflection",
313     "linked_learning_point": "Q52"
314 },
315 {
316     "filename": "Q53.jpg",
317     "location": "Nearby surfaces of EinScan SP 3D Scanner ",
318     "description": "Fixed scan mode uses manual alignment, cannot use automatic
319                   coded markers",
320     "linked_learning_point": "Q53"
321 },
322 {
323     "filename": "Q54.jpg",
324     "location": "Nearby surfaces of EinScan SP 3D Scanner ",
325     "description": "Disadvantage of texture scanning is large data volume and slow
326                   processing, but it can record color information",
327     "linked_learning_point": "Q54"
328 },
329 {
330     "filename": "Q55.jpg",
331     "location": "Nearby surfaces of EinScan SP 3D Scanner ",
332     "description": "EinScan SP 3D Scanner recommended scanning distance is 290-480
333                   mm",
334     "linked_learning_point": "Q55"
335 },
336 {
337     "filename": "Q56.jpg",
338     "location": "Nearby surfaces of EinScan SP 3D Scanner ",
339     "description": "Do not obstruct the path between the light source and the
340                   object",
341     "linked_learning_point": "Q56"
342 },
343 {
344     "filename": "Q57.jpg",
345     "location": "Nearby surfaces of EinScan SP 3D Scanner ",

```

```

521     341     "description": "Avoid looking directly at the light source during scanning",
522     342     "linked_learning_point": "Q57"
523     343 },
524     344 {
525     345     "filename": "Q58.jpg",
526     346     "location": "Nearby surfaces of Trotec Speedy 400 Laser Cutter ",
527     347     "description": "The focusing tool must touch the material surface",
528     348     "linked_learning_point": "Q58"
529     349 },
530     350 {
531     351     "filename": "Q59.jpg",
532     352     "location": "Nearby surfaces of Trotec Speedy 400 Laser Cutter ",
533     353     "description": "Wait for smoke to clear before opening the lid after cutting",
534     354     "linked_learning_point": "Q59"
535     355 },
536     356 {
537     357     "filename": "Q60.jpg",
538     358     "location": "Nearby surfaces of Trotec Speedy 400 Laser Cutter ",
539     359     "description": "Operating procedure sequence",
540     360     "linked_learning_point": "Q60"
541     361 },
542     362 {
543     363     "filename": "Q61.jpg",
544     364     "location": "Nearby surfaces of Trotec Speedy 400 Laser Cutter ",
545     365     "description": "Uncleaned slag causes focus deviation",
546     366     "linked_learning_point": "Q61"
547     367 },
548     368 {
549     369     "filename": "Q62.jpg",
550     370     "location": "Nearby surfaces of Trotec Speedy 400 Laser Cutter ",
551     371     "description": "Laser automatically cuts off when the lid is opened",
552     372     "linked_learning_point": "Q62"
553     373 },
554     374 {
555     375     "filename": "Q63.jpg",
556     376     "location": "Nearby surfaces of Trotec Speedy 400 Laser Cutter ",
557     377     "description": "Exhaust turned off leads to lens contamination and laser beam
558     378     scattering",
559     379     "linked_learning_point": "Q63"
560     379 },
561
562
563
564
565
566
567
568
569
570
571
572

```

```

380  {
381      "filename": "Q64.jpg",
382      "location": "Nearby surfaces of Trotec Speedy 400 Laser Cutter ",
383      "description": "Do not process materials containing chlorine, such as PVC",
384      "linked_learning_point": "Q64"
385  },
386  {
387      "filename": "Q65.jpg",
388      "location": "Nearby surfaces of Trotec Speedy 400 Laser Cutter ",
389      "description": "Laser wavelength is 10.6 micrometers",
390      "linked_learning_point": "Q65"
391  },
392  {
393      "filename": "Q66.jpg",
394      "location": "Nearby surfaces of Trotec Speedy 400 Laser Cutter ",
395      "description": "CO2 laser is best absorbed by organic non-metals like acrylic
396                  and wood",
397      "linked_learning_point": "Q66"
398  },
399  {
400      "filename": "Q67.jpg",
401      "location": "Nearby surfaces of Trotec Speedy 400 Laser Cutter ",
402      "description": "Focus deviation affects cutting quality",
403      "linked_learning_point": "Q67"
404  },
405  {
406      "filename": "Q68.jpg",
407      "location": "Nearby surfaces of Trotec Speedy 400 Laser Cutter ",
408      "description": "Pay attention to connecting the exhaust pipe to avoid
409                  triggering the smoke alarm",
410      "linked_learning_point": "Q68"
411  },
412  {
413      "filename": "Q69.jpg",
414      "location": "Nearby surfaces of Trotec Speedy 400 Laser Cutter ",
415      "description": "In case of danger, press the emergency stop button",
416      "linked_learning_point": "Q69"
417  },
418  {
419      "filename": "R1.gif",

```

```

625     418     "location": "Nearby surfaces of any equipment",
626     419     "description": "Prohibit dangerous operations and behaviors",
627     420     "linked_learning_point": "R1"
628
629     421 },
630
631     422 {
632     423     "filename": "R2.gif",
633     424     "location": "Nearby surfaces of any equipment",
634     425     "description": "Pay attention to important matters",
635     426     "linked_learning_point": "R2"
636
637     427 },
638
639     428 {
640     429     "filename": "R3.gif",
641     430     "location": "On any equipment",
642     431     "description": "Projected holo light highlight to emphasize item",
643     432     "linked_learning_point": "R3"
644
645     433 },
646
647     434 {
648     435     "filename": "R4.gif",
649     436     "location": "On any equipment",
650     437     "description": "Projected light ring highlight to emphasize item",
651     438     "linked_learning_point": "R4"
652
653     439 },
654
655     440 {
656     441     "filename": "R5.gif",
657     442     "location": "Nearby surfaces of any equipment",
658     443     "description": "Arrow pointing down",
659     444     "linked_learning_point": "R5"
660
661     445 },
662
663     446 {
664     447     "filename": "R6.gif",
665     448     "location": "Nearby surfaces of any equipment",
666     449     "description": "Arrow pointing right",
667     450     "linked_learning_point": "R6"
668
669     451 },
670
671     452 {
672     453     "filename": "R7.gif",
673     454     "location": "Nearby surfaces of any equipment",
674     455     "description": "Move left",
675     456     "linked_learning_point": "R7"
676     457 },

```

```
458 {  
459   "filename": "R8.gif",  
460   "location": "Nearby surfaces of any equipment",  
461   "description": "Move right",  
462   "linked_learning_point": "R8"  
463 }  
464 ]
```
